# Supplementary material for: The first PDF moments for three dynamical flavors in Baryon Chiral Perturbation Theory
Source: arXiv:1105.6000 ancillary file (2012-02-16)
Supplement: Supplementary file 1 [file supplement.pdf]

# The first PDF moments for three dynamical flavors in Baryon Chiral Perturbation Theory (Supplement)

Peter C. Bruns, Ludwig Greil, Andreas Schäfer
*Institut für Theoretische Physik, Universität Regensburg, D-93040 Regensburg, Germany*

## Remark

These notes are intended as a supplement to our forthcoming publication on the subject[1]. We present the results of a calculation of generalized baryon form factors in the framework of three-flavor covariant baryon chiral perturbation theory at leading one-loop order.

# 1 Generalized baryon form factors

The generalized baryon form factors are accessible through calculation of baryon matrix elements of totally symmetrized and traceless local operators ($q = u, d, s$)

$$\mathcal{O}^q_{\mu\nu} = i\bar{q}\gamma_{\{\mu}\overleftrightarrow{D}_{\nu\}}q\,. \tag{1}$$

Here, we have introduced the abbreviations

$$A_{\{\mu}B_{\nu\}} = \frac{1}{2}\left(g_{\alpha\mu}g_{\beta\nu} + g_{\beta\mu}g_{\alpha\nu} - \frac{2}{d}g_{\alpha\beta}g_{\mu\nu}\right)A^\alpha B^\beta, \tag{2}$$

$$\overleftrightarrow{D}_\mu = \frac{1}{2}\left(\overrightarrow{D}_\mu - \overleftarrow{D}_\mu\right), \tag{3}$$

where $d$ represents the space-time dimension. For two light quark flavors and assuming isospin symmetry, this matrix element can be decomposed into said generalized form factors. In the $SU(3)_f$ case, however, one finds five different form factors if one imposes no restrictions on isospin or baryon content. In this work, we analyze the flavor-singlet and the flavor-octet sector, i.e.

$$\mathcal{M}^s_{B'B} = \langle B', s', \mathbf{p}'|i\bar{q}\mathbb{1}\gamma_{\{\mu}\overleftrightarrow{D}_{\nu\}}q|B, s, \mathbf{p}\rangle, \tag{4}$$

$$\mathcal{M}^{v,i}_{B'B} = \langle B', s', \mathbf{p}'|i\bar{q}\lambda^i\gamma_{\{\mu}\overleftrightarrow{D}_{\nu\}}q|B, s, \mathbf{p}\rangle, \tag{5}$$

where the $\lambda^i$ denote the Gell-Mann matrices and $B(B')$ labels the incoming (outgoing) baryon from the lowest-lying baryon octet. The decomposition of these matrix elements is given by

$$\begin{aligned}\mathcal{M}^{s,v}_{B'B} = \bar{u}(p')\Big[&A^{s,v}_{B'B}(\Delta^2)\gamma_{\{\mu}\bar{p}_{\nu\}} - i\frac{B^{s,v}_{B'B}(\Delta^2)}{2\bar{m}}\Delta^\alpha\sigma_{\alpha\{\mu}\bar{p}_{\nu\}} + \frac{C^{s,v}_{B'B}(\Delta^2)}{\bar{m}}\Delta_{\{\mu}\Delta_{\nu\}} \\ &+ \frac{D^{s,v}_{B'B}(\Delta^2)}{2\bar{m}}\bar{p}_{\{\mu}\Delta_{\nu\}} + E^{s,v}_{B'B}(\Delta^2)\gamma_{\{\mu}\Delta_{\nu\}}\Big]u(p).\end{aligned} \tag{6}$$

[1]Peter C. Bruns, Ludwig Greil, Andreas Schäfer, *The first PDF moments for three dynamical flavors in Baryon Chiral Perturbation Theory*, to be published

Here, we have defined $\bar{p} = (p' + p)/2$ and $\Delta = p' - p$. Moreover, $\bar{m} = (m_B + m_{B'})/2$. Taking $\mathcal{P}$-, $\mathcal{C}$- and $\mathcal{T}$-symmetry into account, we find that $A^{s,v}$, $B^{s,v}$ and $C^{s,v}$ are Hermitian $8 \times 8$-matrices in the space of one-baryon channels, whereas $D^{s,v}$ and $E^{s,v}$ are anti-Hermitian. These matrices are directly accessible via $SU(3)_f$ BChPT.

In the following sections, we list our results for the form factors $A^{s,v}_{B'B}$ at vanishing momentum transfer, $\Delta^2 = 0$. In Section 2, we present the chiral representation of the form factors in terms of the loop functions derived in the framework of the Infrared Regularization scheme of Becher and Leutwyler. Explicit expressions for the loop functions appearing there, as well as for the baryon wave function renormalization factors, are given in Section 3. Note that we are assuming isospin symmetry in the following.

## 2 Chiral representations of the form factors $\mathbf{A^{s,v}_{B'B}}$

We show here the nonvanishing matrix elements $A^i_{B'B}(0)$. Note that $A_{BB'} = A^*_{B'B}$ due to the hermiticity of $A$. Moreover, we denote $A^{v,i}(\Delta^2 = 0) \equiv A^i$ for brevity. For the definition of the low-energy constants $t_i$ and the tensor couplings $a_{D,F}$, we refer to our forthcoming publication.

### N→N

The nonvanishing matrix elements for nucleon in-and out-states in the octet sector are

$$
\begin{aligned}
A^3_{pp} = {} & Z_N \frac{a_D + a_F}{2} + \frac{4}{3}\Big[3(t_1 + t_2)(2M_K^2 + M_\pi^2) - 2(2t_3 + 2t_4 - t_7 - t_8)(M_K^2 - M_\pi^2)\Big] \\
& + \frac{I_M(M_\pi)}{(24F_0^2 m_0^2)}\Big[(D+F)(3(a_D + a_F)(D+F) + 8(\Delta a_D + \Delta a_F))M_\pi^2 - 3(a_D + a_F)(4 + (D+F)^2)m_0^2\Big] \\
& + \frac{I_M(M_K)}{(36F_0^2 m_0^2)}\Big[-3(3a_F - 6a_F(D-F)^2 + a_D(3 + 2(D-F)(D+3F)))m_0^2 + 2(-\Delta a_D(D-3F) - 9a_F(D-F)^2 + 3a_D(D-F)(D+3F) \\
& \qquad + 3(D+F)\Delta a_F)M_K^2\Big] \\
& + \frac{I_M(M_\eta)}{(24F_0^2 m_0^2)}(a_D + a_F)(D-3F)^2(m_0^2 - M_\eta^2) \\
& - \frac{I_{MB}(M_\pi)}{(48F_0^2 m_0^2)}(D+F)M_\pi^2(-16(\Delta a_D + \Delta a_F)(4m_0^2 - M_\pi^2) + 3(a_D + a_F)(D+F)(-8m_0^2 + 5M_\pi^2)) \\
& - \frac{I_{MB}(M_K)}{(36F_0^2 m_0^2)}M_K^2\Big[2(D(\Delta a_D - 3\Delta a_F) - 3F(\Delta a_D + \Delta a_F))(4m_0^2 - M_K^2) + 3(D-F)((a_D - 3a_F)D + 3(a_D + a_F)F)(-8m_0^2 + 5M_K^2)\Big] \\
& + \frac{I_{MB}(M_\eta)}{(48F_0^2 m_0^2)}(a_D + a_F)(D-3F)^2 M_\eta^2(-8m_0^2 + 5M_\eta^2) \\
& + \frac{I_{MBB}(0, M_\pi)}{(16F_0^2 m_0^2)}(a_D + a_F)(D+F)^2 M_\pi^2(8m_0^4 - 12m_0^2 M_\pi^2 + 3M_\pi^4) \\
& + \frac{I_{MBB}(0, M_K)}{(12F_0^2 m_0^2)}(D-F)\Big[(a_D - 3a_F)D + 3(a_D + a_F)F\Big]M_K^2(8m_0^4 - 12m_0^2 M_K^2 + 3M_K^4) \\
& - \frac{I_{MBB}(0, M_\eta)}{(48F_0^2 m_0^2)}(a_D + a_F)(D-3F)^2 M_\eta^2(8m_0^4 - 12m_0^2 M_\eta^2 + 3M_\eta^4) \\
& - \frac{(D+F)M_\pi^4}{(2304\pi^2 F_0^2 m_0^4)}\Big[9(a_D + a_F)(D+F)(2m_0^2 - M_\pi^2) + 4(\Delta a_D + \Delta a_F)(6m_0^2 - M_\pi^2)\Big] \\
& + \frac{M_K^4}{(3456\pi^2 F_0^2 m_0^4)}\Big[54a_F(D-F)^2(2m_0^2 - M_K^2) - 18a_D(D^2 + 2DF - 3F^2)(2m_0^2 - M_K^2) + (D(\Delta a_D - 3\Delta a_F) \\
& \qquad - 3F(\Delta a_D + \Delta a_F))(6m_0^2 - M_K^2)\Big] \\
& + \frac{(a_D + a_F)(D-3F)^2(2m_0^2 M_\eta^4 - M_\eta^6)}{(768\pi^2 F_0^2 m_0^4)}\,,
\end{aligned}
\qquad (7)
$$

$$
\begin{aligned}
A^8_{pp} &= -Z_N \frac{a_D - 3a_F}{2\sqrt{3}} - \frac{4}{3\sqrt{3}}\Big[3(t_1 - 3t_2)(2M_K^2 + M_\pi^2) + 2(10t_3 - 6t_4 + t_7 - 3t_8 + 6t_9)(M_K^2 - M_\pi^2)\Big] \\
&+ \frac{I_M(M_\pi)}{(8F_0^2 m_0^2)}\sqrt{3}(a_D - 3a_F)(D+F)^2(-m_0^2 + M_\pi^2) \\
&+ \frac{I_M(M_K)}{(12\sqrt{3}F_0^2 m_0^2)}\Big[(-27a_F + a_D(9 + 8D(D-3F)))m_0^2 + 2(5D\Delta a_D - 4a_D D(D-3F) - 3\Delta a_D F - 3D\Delta a_F + 9F\Delta a_F)M_K^2\Big] \\
&- \frac{I_M(M_\eta)}{(24\sqrt{3}F_0^2 m_0^2)}(a_D - 3a_F)(D-3F)^2(m_0^2 - M_\eta^2) \\
&+ \frac{I_{MB}(M_\pi)}{(16F_0^2 m_0^2)}\sqrt{3}(a_D - 3a_F)(D+F)^2 M_\pi^2(8m_0^2 - 5M_\pi^2) \\
&+ \frac{I_{MB}(M_K)}{(6\sqrt{3}F_0^2 m_0^2)}M_K^2\Big[(5D\Delta a_D - 3\Delta a_D F - 3D\Delta a_F + 9F\Delta a_F)(4m_0^2 - M_K^2) + 2a_D D(D-3F)(-8m_0^2 + 5M_K^2)\Big] \\
&+ \frac{I_{MB}(M_\eta)}{(48\sqrt{3}F_0^2 m_0^2)}(a_D - 3a_F)(D-3F)^2 M_\eta^2(8m_0^2 - 5M_\eta^2) \\
&+ \frac{I_{MBB}(0,M_\pi)}{(16F_0^2 m_0^2)}\sqrt{3}(a_D - 3a_F)(D+F)^2 M_\pi^2(8m_0^4 - 12m_0^2 M_\pi^2 + 3M_\pi^4) \\
&- \frac{I_{MBB}(0,M_K)}{(3\sqrt{3}F_0^2 m_0^2)}a_D D(D-3F)M_K^2(8m_0^4 - 12m_0^2 M_K^2 + 3M_K^4) \\
&+ \frac{I_{MBB}(0,M_\eta)}{(48\sqrt{3}F_0^2 m_0^2)}(a_D - 3a_F)(D-3F)^2 M_\eta^2(8m_0^4 - 12m_0^2 M_\eta^2 + 3M_\eta^4) \\
&- \frac{\sqrt{3}(a_D - 3a_F)(D+F)^2(2m_0^2 M_\pi^4 - M_\pi^6)}{(256\pi^2 F_0^2 m_0^4)} \\
&+ \frac{M_K^4}{(1152\sqrt{3}\pi^2 F_0^2 m_0^4)}\Big[24a_D D(D-3F)(2m_0^2 - M_K^2) - (5D\Delta a_D - 3\Delta a_D F - 3D\Delta a_F + 9F\Delta a_F)(6m_0^2 - M_K^2)\Big] \\
&- \frac{(a_D - 3a_F)(D-3F)^2(2m_0^2 M_\eta^4 - M_\eta^6)}{(768\sqrt{3}\pi^2 F_0^2 m_0^4)}\,,
\end{aligned}
\tag{8}
$$

$$
A^1_{np} = A^3_{pp}\,, \qquad A^2_{np} = iA^3_{pp}\,, \qquad A^3_{nn} = -A^3_{pp}\,, \qquad A^8_{nn} = +A^8_{pp}\,. \tag{9}
$$

# $\Lambda, \Sigma$

$$
\begin{aligned}
A^8_{\Lambda\Lambda} &= -Z_\Lambda \frac{a_D}{\sqrt{3}} - \frac{8}{\sqrt{3}}\Big[2(2t_3 + 2t_7 + t_9)(M_K^2 - M_\pi^2) + t_1(2M_K^2 + M_\pi^2) + 2(M_K^2 - M_\pi^2)\Re(t_{10})\Big] \\
&+ \frac{I_M(M_\pi)}{(\sqrt{3}F_0^2 m_0^2)}a_D D^2(m_0^2 - M_\pi^2) \\
&+ \frac{I_M(M_K)}{(6\sqrt{3}F_0^2 m_0^2)}\Big[(18a_F DF - a_D(-9 + D^2 + 9F^2))m_0^2 + (a_D(D^2 + 9F^2) - 6(3a_F DF + \Delta a_D F + D\Delta a_F))M_K^2\Big] \\
&- \frac{I_M(M_\eta)}{(3\sqrt{3}F_0^2 m_0^2)}a_D D^2(m_0^2 - M_\eta^2) \\
&+ \frac{I_{MB}(M_\pi)}{(2\sqrt{3}F_0^2 m_0^2)}M_\pi^2 a_D D^2(-8m_0^2 + 5M_\pi^2) \\
&+ \frac{I_{MB}(M_K)}{(12\sqrt{3}F_0^2 m_0^4)}M_K^2\Big[(-18a_F DF + a_D(D^2 + 9F^2))m_0^2(8m_0^2 - 5M_K^2) + 12(\Delta a_D F + D\Delta a_F)(-4m_0^4 + m_0^2 M_K^2)\Big] \\
&+ \frac{I_{MB}(M_\eta)}{(6\sqrt{3}F_0^2 m_0^2)}a_D D^2 M_\eta^2(8m_0^2 - 5M_\eta^2) \\
&- \frac{I_{MBB}(0,M_\pi)}{(2\sqrt{3}F_0^2 m_0^2)}a_D D^2 M_\pi^2(8m_0^4 - 12m_0^2 M_\pi^2 + 3M_\pi^4) \\
&+ \frac{I_{MBB}(0,M_K)}{(12\sqrt{3}F_0^2 m_0^2)}M_K^2(-18a_F DF + a_D(D^2 + 9F^2))(8m_0^4 - 12m_0^2 M_K^2 + 3M_K^4) \\
&+ \frac{I_{MBB}(0,M_\eta)}{(6\sqrt{3}F_0^2 m_0^2)}a_D D^2 M_\eta^2(8m_0^4 - 12m_0^2 M_\eta^2 + 3M_\eta^4) \\
&- \frac{1}{16\pi^2}\Big[-\frac{a_D D^2 M_\pi^4}{(\sqrt{3}F_0^2 m_0^2)} + \frac{a_D D^2 M_\pi^6}{(2\sqrt{3}F_0^2 m_0^4)}\Big] \\
&- \frac{1}{16\pi^2}\Big[(2a_D D^2 - 36a_F DF + 18a_D F^2 - 6(\Delta a_D F + D\Delta a_F))\frac{M_K^4}{(12\sqrt{3}F_0^2 m_0^2)} \\
&\qquad + (-a_D D^2 + 18a_F DF + \Delta a_D F - 9a_D F^2 + D\Delta a_F)\frac{M_K^6}{(12\sqrt{3}F_0^2 m_0^4)}\Big] \\
&- \frac{1}{16\pi^2}\Big[\frac{a_D D^2 M_\eta^4}{(3\sqrt{3}F_0^2 m_0^2)} - \frac{a_D D^2 M_\eta^6}{(6\sqrt{3}F_0^2 m_0^4)}\Big]\,,
\end{aligned}
\tag{10}
$$

$$
\begin{aligned}
A^3_{\Sigma^0\Lambda} = {} & \sqrt{Z_\Sigma}\sqrt{Z_\Lambda}\frac{a_D}{\sqrt{3}} + \frac{8}{3\sqrt{3}}\left[3t_1(2M_K^2 + M_\pi^2) - 4(t_3 + t_7)(M_K^2 - M_\pi^2) - 3t_{10}(M_K^2 - M_\pi^2)\right] \\
& + \frac{I_M(M_\pi)}{(3\sqrt{3}F_0^2 m_0^2)}\left[(a_D(-3 + D^2) - 6a_F DF)m_0^2 + (-(a_D D^2) + 6a_F DF + 2\Delta a_D F + 2D\Delta a_F)M_\pi^2\right] \\
& + \frac{I_M(M_K)}{(6\sqrt{3}F_0^2 m_0^2)}\left[-3(2a_F DF + a_D(1 + D^2 - 3F^2))m_0^2 + (3a_D D^2 + 6a_F DF + 2\Delta a_D F - 9a_D F^2 + 2D\Delta a_F)M_K^2\right] \\
& + \frac{I_M(M_\eta)}{(3\sqrt{3}F_0^2 m_0^2)} a_D D^2(-m_0^2 + M_\eta^2) \\
& + \frac{I_{MB}(M_\pi)}{(6\sqrt{3}F_0^2 m_0^2)} M_\pi^2(-4(\Delta a_D F + D\Delta a_F)(-4m_0^2 + M_\pi^2) + D(a_D D - 6a_F F)(-8m_0^2 + 5M_\pi^2)) \\
& + \frac{I_{MB}(M_K)}{(12\sqrt{3}F_0^2 m_0^2)} M_K^2\left[3(2a_F DF + a_D(D^2 - 3F^2))(8m_0^2 - 5M_K^2) - 4(\Delta a_D F + D\Delta a_F)(-4m_0^2 + M_K^2)\right] \\
& + \frac{I_{MB}(M_\eta)}{(6\sqrt{3}F_0^2 m_0^2)} a_D D^2 M_\eta^2(8m_0^2 - 5M_\eta^2) \\
& - \frac{I_{MBB}(0, M_\pi)}{(6\sqrt{3}F_0^2 m_0^2)} M_\pi^2 D(a_D D - 6a_F F)(8m_0^4 - 12m_0^2 M_\pi^2 + 3M_\pi^4) \\
& + \frac{I_{MBB}(0, M_K)}{(4\sqrt{3}F_0^2 m_0^2)} M_K^2(2a_F DF + a_D(D^2 - 3F^2))(8m_0^4 - 12m_0^2 M_K^2 + 3M_K^4) \\
& + \frac{I_{MBB}(0, M_\eta)}{(6\sqrt{3}F_0^2 m_0^2)} a_D D^2 M_\eta^2(8m_0^4 - 12m_0^2 M_\eta^2 + 3M_\eta^4) \\
& - \frac{1}{16\pi^2}\left[(-12a_D D^2 + 72a_F DF + 12(\Delta a_D F + D\Delta a_F))\frac{M_\pi^4}{(36\sqrt{3}F_0^2 m_0^2)} + (6a_D D^2 - 36a_F DF - 2(\Delta a_D F + D\Delta a_F))\frac{M_\pi^6}{(36\sqrt{3}F_0^2 m_0^4)}\right] \\
& - \frac{1}{16\pi^2}\left[(18a_D D^2 + 36a_F DF - 54a_D F^2 + 6(\Delta a_D F + D\Delta a_F))\frac{M_K^4}{(36\sqrt{3}F_0^2 m_0^2)}\right. \\
& \qquad \left. + (-9a_D D^2 - 18a_F DF - \Delta a_D F + 27a_D F^2 - D\Delta a_F)\frac{M_K^6}{(36\sqrt{3}F_0^2 m_0^4)}\right] \\
& - \frac{1}{16\pi^2}\left[\frac{a_D D^2 M_\eta^4}{(3\sqrt{3}F_0^2 m_0^2)} - \frac{a_D D^2 M_\eta^6}{(6\sqrt{3}F_0^2 m_0^4)}\right],
\end{aligned}
\tag{11}
$$

$$
\begin{aligned}
A^3_{\Sigma^+\Sigma^+} = {} & Z_\Sigma a_F + \frac{8}{3}(-4(t_4 + t_8)(M_K^2 - M_\pi^2) + 3t_2(2M_K^2 + M_\pi^2)) \\
& + \frac{I_M(M_\pi)}{(9F_0^2 m_0^2)}\left[3(-2a_D DF + 3a_F(-1 + F^2))m_0^2 + (-9a_F F^2 + 2D(\Delta a_D + 3a_D F) + 6F\Delta a_F)M_\pi^2\right] \\
& + \frac{I_M(M_K)}{(6F_0^2 m_0^2)}\left[3(-2a_D DF + a_F(-1 + D^2 + F^2))m_0^2 + (-3a_F(D^2 + F^2) + 2(D(\Delta a_D + 3a_D F) + F\Delta a_F))M_K^2\right] \\
& + \frac{I_M(M_\eta)}{(3F_0^2 m_0^2)} a_F D^2(m_0^2 - M_\eta^2) \\
& + \frac{I_{MB}(M_\pi)}{(18F_0^2 m_0^2)} M_\pi^2(4(D\Delta a_D + 3F\Delta a_F)(4m_0^2 - M_\pi^2) + 3F(-2a_D D + 3a_F F)(-8m_0^2 + 5M_\pi^2)) \\
& + \frac{I_{MB}(M_K)}{(12F_0^2 m_0^2)} M_K^2(4(D\Delta a_D + F\Delta a_F)(4m_0^2 - M_K^2) + 3(-2a_D DF + a_F(D^2 + F^2))(-8m_0^2 + 5M_K^2)) \\
& + \frac{I_{MB}(M_\eta)}{(6F_0^2 m_0^2)} a_F D^2 M_\eta^2(-8m_0^2 + 5M_\eta^2) \\
& + \frac{I_{MBB}(0, M_\pi)}{(6F_0^2 m_0^2)} M_\pi^2 F(2a_D D - 3a_F F)(8m_0^4 - 12m_0^2 M_\pi^2 + 3M_\pi^4) \\
& + \frac{I_{MBB}(0, M_K)}{(4F_0^2 m_0^2)} M_K^2(-2a_D DF + a_F(D^2 + F^2))(-8m_0^4 + 12m_0^2 M_K^2 - 3M_K^4) \\
& - \frac{I_{MBB}(0, M_\eta)}{(6F_0^2 m_0^2)} a_F D^2 M_\eta^2(8m_0^4 - 12m_0^2 M_\eta^2 + 3M_\eta^4) \\
& - \frac{1}{16\pi^2}\left[(12D\Delta a_D + 72a_D DF - 108a_F F^2 + 36F\Delta a_F)\frac{M_\pi^4}{(108F_0^2 m_0^2)} + (-2D\Delta a_D - 36a_D DF + 54a_F F^2 - 6F\Delta a_F)\frac{M_\pi^6}{(108F_0^2 m_0^4)}\right] \\
& - \frac{1}{16\pi^2}\left[(-54a_F D^2 + 18D\Delta a_D + 108a_D DF - 54a_F F^2 + 18F\Delta a_F)\frac{M_K^4}{(108F_0^2 m_0^2)}\right. \\
& \qquad \left. + (27a_F D^2 - 3D\Delta a_D - 54a_D DF + 27a_F F^2 - 3F\Delta a_F)\frac{M_K^6}{(108F_0^2 m_0^4)}\right] \\
& - \frac{1}{16\pi^2}\left[-\frac{a_F D^2 M_\eta^4}{(3F_0^2 m_0^2)} + \frac{a_F D^2 M_\eta^6}{(6F_0^2 m_0^4)}\right],
\end{aligned}
\tag{12}
$$

$$
\begin{aligned}
A^8_{\Sigma^+\Sigma^+} = {} & Z_\Sigma \frac{a_D}{\sqrt{3}} + \frac{8}{3\sqrt{3}}(-2(2t_3+2t_7+3t_9)(M_K^2-M_\pi^2)+3t_1(2M_K^2+M_\pi^2)) \\
& - \frac{I_M(M_\pi)}{(3\sqrt{3}F_0^2m_0^2)} a_D(D^2-6F^2)(m_0^2-M_\pi^2) \\
& + \frac{I_M(M_K)}{(2\sqrt{3}F_0^2m_0^2)}\Big[-(6a_FDF+a_D(3+D^2+F^2))m_0^2+(a_D(D^2+F^2)+2(3a_FDF+\Delta a_DF+D\Delta a_F))M_K^2\Big] \\
& + \frac{I_M(M_\eta)}{(3\sqrt{3}F_0^2m_0^2)} a_D D^2(m_0^2-M_\eta^2) \\
& + \frac{I_{MB}(M_\pi)}{(6\sqrt{3}F_0^2m_0^2)} M_\pi^2 a_D(D^2-6F^2)(8m_0^2-5M_\pi^2) \\
& - \frac{I_{MB}(M_K)}{(4\sqrt{3}F_0^2m_0^4)} M_K^2((6a_FDF+a_D(D^2+F^2))m_0^2(-8m_0^2+5M_K^2)+4(\Delta a_DF+D\Delta a_F)(-4m_0^4+m_0^2M_K^2)) \\
& + \frac{I_{MB}(M_\eta)}{(6\sqrt{3}F_0^2m_0^2)} a_D D^2 M_\eta^2(-8m_0^2+5M_\eta^2) \\
& + \frac{I_{MBB}(0,M_\pi)}{(6\sqrt{3}F_0^2m_0^2)} M_\pi^2 a_D(D^2-6F^2)(8m_0^4-12m_0^2M_\pi^2+3M_\pi^4) \\
& + \frac{I_{MBB}(0,M_K)}{(4\sqrt{3}F_0^2m_0^2)} M_K^2(6a_FDF+a_D(D^2+F^2))(8m_0^4-12m_0^2M_K^2+3M_K^4) \\
& - \frac{I_{MBB}(0,M_\eta)}{(6\sqrt{3}F_0^2m_0^2)} a_D D^2 M_\eta^2(8m_0^4-12m_0^2M_\eta^2+3M_\eta^4) \\
& - \frac{1}{16\pi^2}\Big[(12D\Delta a_D+72a_DDF-108a_FF^2+36F\Delta a_F)\frac{M_\pi^4}{(108F_0^2m_0^2)}+(-2D\Delta a_D-36a_DDF+54a_FF^2-6F\Delta a_F)\frac{M_\pi^6}{(108F_0^2m_0^4)}\Big] \\
& - \frac{1}{16\pi^2}\Big[(-54a_FD^2+18D\Delta a_D+108a_DDF-54a_FF^2+18F\Delta a_F)\frac{M_K^4}{(108F_0^2m_0^2)} \\
& \qquad +(27a_FD^2-3D\Delta a_D-54a_DDF+27a_FF^2-3F\Delta a_F)\frac{M_K^6}{(108F_0^2m_0^4)}\Big] \\
& - \frac{1}{16\pi^2}\Big[-\frac{a_FD^2M_\eta^4}{(3F_0^2m_0^2)}+\frac{a_FD^2M_\eta^6}{(6F_0^2m_0^4)}\Big]\,.
\end{aligned} \tag{13}
$$

$$
\sqrt{2}A^1_{\Sigma^+\Lambda} = \sqrt{2}A^1_{\Sigma^-\Lambda} = A^3_{\Sigma^0\Lambda}\,, \qquad A^2_{\Sigma^+\Lambda} = -A^2_{\Sigma^-\Lambda} = -iA^1_{\Sigma^+\Lambda}\,, \qquad \sqrt{2}A^1_{\Sigma^0\Sigma^+} = -\sqrt{2}A^1_{\Sigma^0\Sigma^-} = -A^3_{\Sigma^+\Sigma^+}\,, \tag{14}
$$

$$
A^2_{\Sigma^0\Sigma^+} = -A^2_{\Sigma^0\Sigma^-} = iA^1_{\Sigma^0\Sigma^+}\,, \qquad A^3_{\Sigma^-\Sigma^-} = -A^3_{\Sigma^+\Sigma^+}\,, \qquad A^8_{\Sigma^-\Sigma^-} = A^8_{\Sigma^0\Sigma^0} = A^8_{\Sigma^+\Sigma^+}\,. \tag{15}
$$

## $\mathbf{N \to \Lambda, \Sigma}$

$$
\begin{aligned}
A^4_{\Lambda p} = & -\sqrt{Z_\Lambda}\sqrt{Z_N}\frac{a_D + 3a_F}{2\sqrt{6}} \\
& - \frac{2}{3}\sqrt{\frac{2}{3}}(M_K^2 \Big[6t_1 + 18t_2 + 2t_3 + 6t_4 - 6t_5 - 18t_6 + 2t_7 + 6t_8) + M_\pi^2(3t_1 + 9t_2 - 2t_3 - 6t_4 + 6t_5 + 18t_6 - 2t_7 - 6t_8) \\
& \qquad + 6(M_K^2 - M_\pi^2)t_{10}^*\Big] \\
& + \frac{I_M(M_\pi)}{(16\sqrt{6}F_0^2 m_0^2)}\Big[3(a_F(3 - 4D(D+F)) + a_D(1 + 4D(D+F)))m_0^2 \\
& \qquad - 2(3D\Delta a_D + \Delta a_D F + 6a_D D(D+F) - 6a_F D(D+F) + D\Delta a_F + 3F\Delta a_F)M_\pi^2\Big] \\
& + \frac{I_M(M_K)}{(24\sqrt{6}F_0^2 m_0^2)}\Big[(3a_F(9 - 2(D-3F)^2) + a_D(9 - 2(D-3F)(5D-3F)))m_0^2 \\
& \qquad + 2(-5D\Delta a_D + 3a_F(D-3F)^2 + a_D(D-3F)(5D-3F) - 3\Delta a_D F - 3D\Delta a_F - 9F\Delta a_F)M_K^2\Big] \\
& + \frac{I_M(M_\eta)}{(48\sqrt{6}F_0^2 m_0^2)}\Big[-(a_D + 3a_F)(-9 + 4D(D-3F))m_0^2 + 2(2a_D D(D-3F) + 6a_F D(D-3F) - (D+3F)(\Delta a_D + 3\Delta a_F))M_\eta^2\Big] \\
& + \frac{I_{MB}(M_\pi)}{(8\sqrt{6}F_0^2 m_0^2)}M_\pi^2\Big[(D(3\Delta a_D + \Delta a_F) + F(\Delta a_D + 3\Delta a_F))(-4m_0^2 + M_\pi^2) + 3a_D D(D+F)(-8m_0^2 + 5M_\pi^2) \\
& \qquad + 3a_F D(D+F)(8m_0^2 - 5M_\pi^2)\Big] \\
& + \frac{I_{MB}(M_K)}{(24\sqrt{6}F_0^2 m_0^2)}M_K^2\Big[(D-3F)(5a_D D + 3a_F D - 3a_D F - 9a_F F)(8m_0^2 - 5M_K^2) \\
& \qquad - 2(5D\Delta a_D + 3\Delta a_D F + 3D\Delta a_F + 9F\Delta a_F)(4m_0^2 - M_K^2)\Big] \\
& + \frac{I_{MB}(M_\eta)}{(24\sqrt{6}F_0^2 m_0^2)}M_\eta^2\Big[(a_D + 3a_F)D(D-3F)(8m_0^2 - 5M_\eta^2) - (D+3F)(\Delta a_D + 3\Delta a_F)(4m_0^2 - M_\eta^2)\Big] \\
& - \frac{I_{MBB}(0, M_\pi)}{(8F_0^2 m_0^2)}\sqrt{\frac{3}{2}}M_\pi^2(a_D - a_F)D(D+F)(8m_0^4 - 12m_0^2 M_\pi^2 + 3M_\pi^4) \\
& + \frac{I_{MBB}(0, M_K)}{(24\sqrt{6}F_0^2 m_0^2)}M_K^2(D-3F)(5a_D D + 3a_F D - 3a_D F - 9a_F F)(8m_0^4 - 12m_0^2 M_K^2 + 3M_K^4) \\
& + \frac{I_{MBB}(0, M_\eta)}{(24\sqrt{6}F_0^2 m_0^2)}M_\eta^2(a_D + 3a_F)D(D-3F)(8m_0^4 - 12m_0^2 M_\eta^2 + 3M_\eta^4) \\
& - \frac{1}{16\pi^2}\Big[(-54D\Delta a_D - 18\Delta a_D F - 216(a_D - a_F)D(D+F) - 18D\Delta a_F - 54F\Delta a_F)\frac{M_\pi^4}{(288\sqrt{6}F_0^2 m_0^2)} \\
& \qquad + (9D\Delta a_D + 3\Delta a_D F + 108(a_D - a_F)D(D+F) + 3D\Delta a_F + 9F\Delta a_F)\frac{M_\pi^6}{(288\sqrt{6}F_0^2 m_0^4)}\Big] \\
& - \frac{1}{16\pi^2}\Big[(-60D\Delta a_D - 36\Delta a_D F + 24(D-3F)(5a_D D + 3a_F D - 3a_D F - 9a_F F) - 36D\Delta a_F - 108F\Delta a_F)\frac{M_K^4}{(288\sqrt{6}F_0^2 m_0^2)} \\
& \qquad + (10D\Delta a_D + 6\Delta a_D F - 12(D-3F)(5a_D D + 3a_F D - 3a_D F - 9a_F F) + 6D\Delta a_F + 18F\Delta a_F)\frac{M_K^6}{(288\sqrt{6}F_0^2 m_0^4)}\Big] \\
& - \frac{1}{16\pi^2}\Big[(-6D\Delta a_D + 24(a_D + 3a_F)D(D-3F) - 18\Delta a_D F - 18D\Delta a_F - 54F\Delta a_F)\frac{M_\eta^4}{(288\sqrt{6}F_0^2 m_0^2)} \\
& \qquad + (D\Delta a_D - 12(a_D + 3a_F)D(D-3F) + 3\Delta a_D F + 3D\Delta a_F + 9F\Delta a_F)\frac{M_\eta^6}{(288\sqrt{6}F_0^2 m_0^4)}\Big],
\end{aligned}
\tag{16}
$$

$$
\begin{aligned}
A^6_{\Sigma^+ p} = & \sqrt{Z_\Sigma}\sqrt{Z_N}\frac{a_D - a_F}{2} + \frac{4}{3}\Big[2(t_3 - t_4 - 3t_5 + 3t_6 + t_7 - t_8)(M_K^2 - M_\pi^2) + 3(t_1 - t_2)(2M_K^2 + M_\pi^2)\Big] \\
& + \frac{I_M(M_\pi)}{(144F_0^2 m_0^2)}\Big[ - 3(a_D(9 + 4(D - 6F)(D + F)) + 3a_F(-3 + 4(D + F)(D + 2F)))m_0^2 \\
& \qquad + 2(-D\Delta a_D + 9\Delta a_D F + 6a_D(D - 6F)(D + F) + 18a_F(D + F)(D + 2F) + 9D\Delta a_F - 9F\Delta a_F)M_\pi^2\Big] \\
& + \frac{I_M(M_K)}{(72F_0^2 m_0^2)}\Big[ - 3(-9a_F + 6a_F(D + F)^2 + a_D(9 + 2(D - 3F)(D + F)))m_0^2 \\
& \qquad + 2(-5D\Delta a_D + 9\Delta a_D F + 3a_D(D - 3F)(D + F) + 9a_F(D + F)^2 + 9D\Delta a_F - 9F\Delta a_F)M_K^2\Big] \\
& + \frac{I_M(M_\eta)}{(48F_0^2 m_0^2)}\Big[-(a_D - a_F)(9 + 4D(D - 3F))m_0^2 + 2(2a_D D(D - 3F) - 2a_F D(D - 3F) - 3(D - F)(\Delta a_D - \Delta a_F))M_\eta^2\Big] \\
& + \frac{I_{MB}(M_\pi)}{(72F_0^2 m_0^2)}M_\pi^2\Big[3a_D(D - 6F)(D + F)(8m_0^2 - 5M_\pi^2) + 9a_F(D + F)(D + 2F)(8m_0^2 - 5M_\pi^2) \\
& \qquad + (D(\Delta a_D - 9\Delta a_F) + 9F(-\Delta a_D + \Delta a_F))(-4m_0^2 + M_\pi^2)\Big] \\
& - \frac{I_{MB}(M_K)}{(72F_0^2 m_0^2)}M_K^2\Big[2(5D\Delta a_D - 9\Delta a_D F - 9D\Delta a_F + 9F\Delta a_F)(4m_0^2 - M_K^2) \\
& \qquad + 3(D + F)(a_D(D - 3F) + 3a_F(D + F))(-8m_0^2 + 5M_K^2)\Big] \\
& - \frac{I_{MB}(M_\eta)}{(24F_0^2 m_0^2)}M_\eta^2\Big[3(D - F)(\Delta a_D - \Delta a_F)(4m_0^2 - M_\eta^2) + (a_D - a_F)D(D - 3F)(-8m_0^2 + 5M_\eta^2)\Big] \\
& + \frac{I_{MBB}(0, M_\pi)}{(24F_0^2 m_0^2)}M_\pi^2(D + F)(a_D(D - 6F) + 3a_F(D + 2F))(8m_0^4 - 12m_0^2 M_\pi^2 + 3M_\pi^4) \\
& + \frac{I_{MBB}(0, M_K)}{(24F_0^2 m_0^2)}M_K^2(D + F)(a_D(D - 3F) + 3a_F(D + F))(8m_0^4 - 12m_0^2 M_K^2 + 3M_K^4) \\
& + \frac{I_{MBB}(0, M_\eta)}{(24F_0^2 m_0^2)}M_\eta^2(a_D - a_F)D(D - 3F)(8m_0^4 - 12m_0^2 M_\eta^2 + 3M_\eta^4) \\
& - \frac{1}{16\pi^2}\Big[(-6D\Delta a_D + 54\Delta a_D F + 72(D + F)(a_D(D - 6F) + 3a_F(D + 2F)) + 54D\Delta a_F - 54F\Delta a_F)\frac{M_\pi^4}{(864F_0^2 m_0^2)} \\
& \qquad + (D\Delta a_D - 9\Delta a_D F - 36(D + F)(a_D(D - 6F) + 3a_F(D + 2F)) - 9D\Delta a_F + 9F\Delta a_F)\frac{M_\pi^6}{(864F_0^2 m_0^4)}\Big] \\
& - \frac{1}{16\pi^2}\Big[(-60D\Delta a_D + 108\Delta a_D F + 72(D + F)(a_D(D - 3F) + 3a_F(D + F)) + 108D\Delta a_F - 108F\Delta a_F)\frac{M_K^4}{(864F_0^2 m_0^2)} \\
& \qquad + (10D\Delta a_D - 18\Delta a_D F - 36(D + F)(a_D(D - 3F) + 3a_F(D + F)) - 18D\Delta a_F + 18F\Delta a_F)\frac{M_K^6}{(864F_0^2 m_0^4)}\Big] \\
& - \frac{1}{16\pi^2}\Big[(-54D\Delta a_D + 72(a_D - a_F)D(D - 3F) + 54\Delta a_D F + 54D\Delta a_F - 54F\Delta a_F)\frac{M_\eta^4}{(864F_0^2 m_0^2)} \\
& \qquad + (9D\Delta a_D - 36(a_D - a_F)D(D - 3F) - 9\Delta a_D F - 9D\Delta a_F + 9F\Delta a_F)\frac{M_\eta^6}{(864F_0^2 m_0^4)}\Big],
\end{aligned} \tag{17}
$$

$$
\begin{aligned}
A^{6}_{\Sigma^+ p} = {} & \sqrt{Z_\Sigma}\sqrt{Z_N}\,\frac{a_D - a_F}{2} + \frac{4}{3}\Big[(2(t_3 - t_4 - 3t_5 + 3t_6 + t_7 - t_8)(M_K^2 - M_\pi^2) + 3(t_1 - t_2)(2M_K^2 + M_\pi^2)\Big] \\
& + \frac{I_M(M_\pi)}{(144F_0^2 m_0^2)}\Big[ - 3(a_D(9 + 4(D - 6F)(D + F)) + 3a_F(-3 + 4(D + F)(D + 2F)))m_0^2 \\
& \qquad + 2(-D\Delta a_D + 9\Delta a_D F + 6a_D(D - 6F)(D + F) + 18a_F(D + F)(D + 2F) + 9D\Delta a_F - 9F\Delta a_F)M_\pi^2\Big] \\
& + \frac{I_M(M_K)}{(72F_0^2 m_0^2)}\Big[ - 3(-9a_F + 6a_F(D + F)^2 + a_D(9 + 2(D - 3F)(D + F)))m_0^2 \\
& \qquad + 2(-5D\Delta a_D + 9\Delta a_D F + 3a_D(D - 3F)(D + F) + 9a_F(D + F)^2 + 9D\Delta a_F - 9F\Delta a_F)M_K^2\Big] \\
& + \frac{I_M(M_\eta)}{(48F_0^2 m_0^2)}\Big[-(a_D - a_F)(9 + 4D(D - 3F))m_0^2 + 2(2a_D D(D - 3F) - 2a_F D(D - 3F) - 3(D - F)(\Delta a_D - \Delta a_F))M_\eta^2\Big] \\
& + \frac{I_{MB}(M_\pi)}{(72F_0^2 m_0^2)}M_\pi^2\Big[3a_D(D - 6F)(D + F)(8m_0^2 - 5M_\pi^2) + 9a_F(D + F)(D + 2F)(8m_0^2 - 5M_\pi^2) \\
& \qquad + (D(\Delta a_D - 9\Delta a_F) + 9F(-\Delta a_D + \Delta a_F))(-4m_0^2 + M_\pi^2)\Big] \\
& - \frac{I_{MB}(M_K)}{(72F_0^2 m_0^2)}M_K^2\Big[2(5D\Delta a_D - 9\Delta a_D F - 9D\Delta a_F + 9F\Delta a_F)(4m_0^2 - M_K^2) \\
& \qquad + 3(D + F)(a_D(D - 3F) + 3a_F(D + F))(-8m_0^2 + 5M_K^2)biggr] \\
& - \frac{I_{MB}(M_\eta)}{(24F_0^2 m_0^2)}M_\eta^2(3(D - F)(\Delta a_D - \Delta a_F)(4m_0^2 - M_\eta^2) + (a_D - a_F)D(D - 3F)(-8m_0^2 + 5M_\eta^2)) \\
& + \frac{I_{MBB}(0, M_\pi)}{(24F_0^2 m_0^2)}M_\pi^2(D + F)(a_D(D - 6F) + 3a_F(D + 2F))(8m_0^4 - 12m_0^2 M_\pi^2 + 3M_\pi^4) \\
& + \frac{I_{MBB}(0, M_K)}{(24F_0^2 m_0^2)}M_K^2(D + F)(a_D(D - 3F) + 3a_F(D + F))(8m_0^4 - 12m_0^2 M_K^2 + 3M_K^4) \\
& + \frac{I_{MBB}(0, M_\eta)}{(24F_0^2 m_0^2)}M_\eta^2(a_D - a_F)D(D - 3F)(8m_0^4 - 12m_0^2 M_\eta^2 + 3M_\eta^4) \\
& - \frac{1}{16\pi^2}\Big[(-6D\Delta a_D + 54\Delta a_D F + 72(D + F)(a_D(D - 6F) + 3a_F(D + 2F)) + 54D\Delta a_F - 54F\Delta a_F)\frac{M_\pi^4}{(864F_0^2 m_0^2)} \\
& \qquad + (D\Delta a_D - 9\Delta a_D F - 36(D + F)(a_D(D - 6F) + 3a_F(D + 2F)) - 9D\Delta a_F + 9F\Delta a_F)\frac{M_\pi^6}{(864F_0^2 m_0^4)}\Big] \\
& - \frac{1}{16\pi^2}\Big[(-60D\Delta a_D + 108\Delta a_D F + 72(D + F)(a_D(D - 3F) + 3a_F(D + F)) + 108D\Delta a_F - 108F\Delta a_F)\frac{M_K^4}{(864F_0^2 m_0^2)} \\
& \qquad + (10D\Delta a_D - 18\Delta a_D F - 36(D + F)(a_D(D - 3F) + 3a_F(D + F)) - 18D\Delta a_F + 18F\Delta a_F)\frac{M_K^6}{(864F_0^2 m_0^4)}\Big] \\
& - \frac{1}{16\pi^2}\Big[(-54D\Delta a_D + 72(a_D - a_F)D(D - 3F) + 54\Delta a_D F + 54D\Delta a_F - 54F\Delta a_F)\frac{M_\eta^4}{(864F_0^2 m_0^2)} \\
& \qquad + (9D\Delta a_D - 36(a_D - a_F)D(D - 3F) - 9\Delta a_D F - 9D\Delta a_F + 9F\Delta a_F)\frac{M_\eta^6}{(864F_0^2 m_0^4)}\Big] ,
\end{aligned}
\tag{18}
$$

$$
A^5_{\Lambda p} = iA^4_{\Lambda p}\,, \qquad A^7_{\Sigma^+ p} = iA^6_{\Sigma^+ p}\,, \qquad \sqrt{2}A^4_{\Sigma^0 p} = A^6_{\Sigma^+ p}\,, \qquad A^5_{\Sigma^0 p} = iA^4_{\Sigma^0 p}\,, \tag{19}
$$

$$
A^6_{\Lambda n} = A^4_{\Lambda p}\,, \qquad A^7_{\Lambda n} = iA^6_{\Lambda n}\,, \qquad A^4_{\Sigma^- n} = A^6_{\Sigma^+ p}\,, \qquad A^5_{\Sigma^- n} = iA^4_{\Sigma^- n}\,, \qquad A^6_{\Sigma^0 n} = -iA^7_{\Sigma^0 n} = -A^4_{\Sigma^0 p}\,. \tag{20}
$$

## $\mathbf{\Lambda, \Sigma \to \Xi}$

$$
\begin{aligned}
A^{6}_{\Xi^0\Lambda} = & -\sqrt{Z_\Xi}\sqrt{Z_\Lambda}\frac{a_D - 3a_F}{2\sqrt{6}} \\
& - \frac{2}{3}\sqrt{\frac{2}{3}}\Big[M_K^2(6t_1 - 18t_2 + 2t_3 - 6t_4 - 6t_5 + 18t_6 + 20t_7 - 12t_8) + M_\pi^2(3t_1 - 9t_2 - 2t_3 + 6t_4 + 6t_5 - 18t_6 - 20t_7 + 12t_8) \\
& \quad + 6t_{10}(M_K^2 - M_\pi^2)\Big] \\
& + \frac{I_M(M_\pi)}{(16\sqrt{6}F_0^2 m_0^2)}\Big[3(a_D - 3a_F + 4a_D D^2 + 4a_F D^2 - 4(a_D + a_F)DF)m_0^2 \\
& \quad - 2(-3D\Delta a_D + 6a_D D(D-F) + 6a_F D(D-F) + \Delta a_D F + D\Delta a_F - 3F\Delta a_F)M_\pi^2\Big] \\
& + \frac{I_M(M_K)}{(24\sqrt{6}F_0^2 m_0^2)}\Big[(3a_F(-9 + 2(D+3F)^2) - a_D(-9 + 2(D+3F)(5D+3F)))m_0^2 \\
& \quad + 2(5D\Delta a_D - 3\Delta a_D F - 3a_F(D+3F)^2 + a_D(D+3F)(5D+3F) - 3D\Delta a_F + 9F\Delta a_F)M_K^2\Big] \\
& + \frac{I_M(M_\eta)}{(48\sqrt{6}F_0^2 m_0^2)}\Big[-(a_D - 3a_F)(-9 + 4D(D+3F))m_0^2 + 2(2a_D D(D+3F) - 6a_F D(D+3F) + (D-3F)(\Delta a_D - 3\Delta a_F))M_\eta^2\Big] \\
& + \frac{I_{MB}(M_\pi)}{(8\sqrt{6}F_0^2 m_0^2)}M_\pi^2\Big[(3D\Delta a_D - \Delta a_D F - D\Delta a_F + 3F\Delta a_F)(4m_0^2 - M_\pi^2) + 3a_D D(D-F)(-8m_0^2 + 5M_\pi^2) \\
& \quad + 3a_F D(D-F)(-8m_0^2 + 5M_\pi^2)\Big] \\
& + \frac{I_{MB}(M_K)}{(24\sqrt{6}F_0^2 m_0^2)}M_K^2\Big[(D+3F)(-3a_F(D+3F) + a_D(5D+3F))(8m_0^2 - 5M_K^2) \\
& \quad + 2(5D\Delta a_D - 3\Delta a_D F - 3D\Delta a_F + 9F\Delta a_F)(4m_0^2 - M_K^2)\Big] \\
& + \frac{I_{MB}(M_\eta)}{(24\sqrt{6}F_0^2 m_0^2)}M_\eta^2((a_D - 3a_F)D(D+3F)(8m_0^2 - 5M_\eta^2) + (D-3F)(\Delta a_D - 3\Delta a_F)(4m_0^2 - M_\eta^2)) \\
& - \frac{I_{MBB}(0, M_\pi)}{(8F_0^2 m_0^2)}\sqrt{\frac{3}{2}}M_\pi^2(a_D + a_F)D(D-F)(8m_0^4 - 12m_0^2 M_\pi^2 + 3M_\pi^4) \\
& + \frac{I_{MBB}(0, M_K)}{(24\sqrt{6}F_0^2 m_0^2)}M_K^2(D+3F)(-3a_F(D+3F) + a_D(5D+3F))(8m_0^4 - 12m_0^2 M_K^2 + 3M_K^4) \\
& + \frac{I_{MBB}(0, M_\eta)}{(24\sqrt{6}F_0^2 m_0^2)}M_\eta^2(a_D - 3a_F)D(D+3F)(8m_0^4 - 12m_0^2 M_\eta^2 + 3M_\eta^4) \\
& - \frac{1}{16\pi^2}\Big[(54D\Delta a_D - 216(a_D + a_F)D(D-F) - 18\Delta a_D F - 18D\Delta a_F + 54F\Delta a_F)\frac{M_\pi^4}{(288\sqrt{6}F_0^2 m_0^2)} \\
& \quad + (-9D\Delta a_D + 108(a_D + a_F)D(D-F) + 3\Delta a_D F + 3D\Delta a_F - 9F\Delta a_F)\frac{M_\pi^6}{(288\sqrt{6}F_0^2 m_0^4)}\Big] \\
& - \frac{1}{16\pi^2}\Big[(60D\Delta a_D - 36\Delta a_D F + 24(D+3F)(-3a_F(D+3F) + a_D(5D+3F)) - 36D\Delta a_F + 108F\Delta a_F)\frac{M_K^4}{(288\sqrt{6}F_0^2 m_0^2)} \\
& \quad + (-10D\Delta a_D + 6\Delta a_D F + 12(D+3F)(-5a_D D + 3a_F D - 3a_D F + 9a_F F) + 6D\Delta a_F - 18F\Delta a_F)\frac{M_K^6}{(288\sqrt{6}F_0^2 m_0^4)}\Big] \\
& - \frac{1}{16\pi^2}\Big[(6D\Delta a_D - 18\Delta a_D F + 24(a_D - 3a_F)D(D+3F) - 18D\Delta a_F + 54F\Delta a_F)\frac{M_\eta^4}{(288\sqrt{6}F_0^2 m_0^2)} \\
& \quad + (-D\Delta a_D + 3\Delta a_D F - 12(a_D - 3a_F)D(D+3F) + 3D\Delta a_F - 9F\Delta a_F)\frac{M_\eta^6}{(288\sqrt{6}F_0^2 m_0^4)}\Big],
\end{aligned}
\tag{21}
$$

$$
\begin{aligned}
A^4_{\Xi^0\Sigma^+} =& \sqrt{Z_\Xi}\sqrt{Z_\Sigma}\frac{a_D+a_F}{2} + \frac{4}{3}\Big[2(t_3+t_4-3t_5-3t_6-2t_7-2t_8)(M_K^2-M_\pi^2)+3(t_1+t_2)(2M_K^2+M_\pi^2)\Big] \\
&+ \frac{I_M(M_\pi)}{(144F_0^2m_0^2)}\Big[-3(3a_F(3-4(D-2F)(D-F))+a_D(9+4(D-F)(D+6F)))m_0^2 \\
&\qquad +2(-18a_F(D-2F)(D-F)+6a_D(D-F)(D+6F)+\Delta a_D(D+9F)+9(D+F)\Delta a_F)M_\pi^2\Big] \\
&+ \frac{I_M(M_K)}{(72F_0^2m_0^2)}\Big[-3(9a_F-6a_F(D-F)^2+a_D(9+2(D-F)(D+3F)))m_0^2 \\
&\qquad +2(-9a_F(D-F)^2+3a_D(D-F)(D+3F)+\Delta a_D(5D+9F)+9(D+F)\Delta a_F)M_K^2\Big] \\
&+ \frac{I_M(M_\eta)}{(48F_0^2m_0^2)}\Big[-(a_D+a_F)(9+4D(D+3F))m_0^2+2(2a_DD(D+3F)+2a_FD(D+3F)+3(D+F)(\Delta a_D+\Delta a_F))M_\eta^2\Big] \\
&+ \frac{I_{MB}(M_\pi)}{(72F_0^2m_0^2)}M_\pi^2\Big[-9a_F(D-2F)(D-F)(8m_0^2-5M_\pi^2)+3a_D(D-F)(D+6F)(8m_0^2-5M_\pi^2) \\
&\qquad +(\Delta a_D(D+9F)+9(D+F)\Delta a_F)(4m_0^2-M_\pi^2)\Big] \\
&- \frac{I_{MB}(M_K)}{(72F_0^2m_0^2)}M_K^2\Big[-2(9F(\Delta a_D+\Delta a_F)+D(5\Delta a_D+9\Delta a_F))(4m_0^2-M_K^2) \\
&\qquad +3(D-F)((a_D-3a_F)D+3(a_D+a_F)F)(-8m_0^2+5M_K^2)\Big] \\
&- \frac{I_{MB}(M_\eta)}{(24F_0^2m_0^2)}M_\eta^2\Big[-3(D+F)(\Delta a_D+\Delta a_F)(4m_0^2-M_\eta^2)+(a_D+a_F)D(D+3F)(-8m_0^2+5M_\eta^2)\Big] \\
&+ \frac{I_{MBB}(0,M_\pi)}{(24F_0^2m_0^2)}M_\pi^2(D-F)((a_D-3a_F)D+6(a_D+a_F)F)(8m_0^4-12m_0^2M_\pi^2+3M_\pi^4) \\
&+ \frac{I_{MBB}(0,M_K)}{(24F_0^2m_0^2)}M_K^2(D-F)((a_D-3a_F)D+3(a_D+a_F)F)(8m_0^4-12m_0^2M_K^2+3M_K^4) \\
&+ \frac{I_{MBB}(0,M_\eta)}{(24F_0^2m_0^2)}M_\eta^2(a_D+a_F)D(D+3F)(8m_0^4-12m_0^2M_\eta^2+3M_\eta^4) \\
&- \frac{1}{16\pi^2}\Big[(6D\Delta a_D+54\Delta a_DF+72(D-F)(a_DD-3a_FD+6a_DF+6a_FF)+54D\Delta a_F+54F\Delta a_F)\frac{M_\pi^4}{(864F_0^2m_0^2)} \\
&\qquad +(-D\Delta a_D-9\Delta a_DF-36(D-F)(a_DD-3a_FD+6a_DF+6a_FF)-9D\Delta a_F-9F\Delta a_F)\frac{M_\pi^6}{(864F_0^2m_0^4)}\Big] \\
&- \frac{1}{16\pi^2}\Big[(60D\Delta a_D+108\Delta a_DF+72(D-F)(3a_F(-D+F)+a_D(D+3F))+108D\Delta a_F+108F\Delta a_F)\frac{M_K^4}{(864F_0^2m_0^2)} \\
&\qquad +(-10D\Delta a_D-18\Delta a_DF-36(D-F)(3a_F(-D+F)+a_D(D+3F))-18D\Delta a_F-18F\Delta a_F)\frac{M_K^6}{(864F_0^2m_0^4)}\Big] \\
&- \frac{1}{16\pi^2}\Big[(54D\Delta a_D+54\Delta a_DF+72(a_D+a_F)D(D+3F)+54D\Delta a_F+54F\Delta a_F)\frac{M_\eta^4}{(864F_0^2m_0^2)} \\
&\qquad +(-9D\Delta a_D-9\Delta a_DF-36(a_D+a_F)D(D+3F)-9D\Delta a_F-9F\Delta a_F)\frac{M_\eta^6}{(864F_0^2m_0^4)}\Big]\,.
\end{aligned}
\tag{22}
$$

$$
A^7_{\Xi^0\Lambda} = iA^6_{\Xi^0\Lambda}\,,\qquad A^4_{\Xi^-\Lambda} = A^6_{\Xi^0\Lambda}\,,\qquad -\sqrt{2}A^6_{\Xi^0\Sigma^0} = \sqrt{2}A^4_{\Xi^-\Sigma^0} = A^6_{\Xi^-\Sigma^-} = A^4_{\Xi^0\Sigma^+}\,,\qquad A^7_{\Xi^0\Sigma^0} = iA^6_{\Xi^0\Sigma^0}\,, \tag{23}
$$

$$
A^5_{\Xi^-\Lambda} = iA^4_{\Xi^-\Lambda}\,,\qquad A^5_{\Xi^0\Sigma^+} = iA^4_{\Xi^0\Sigma^+}\,,\qquad A^5_{\Xi^-\Sigma^0} = iA^4_{\Xi^-\Sigma^0}\,,\qquad A^7_{\Xi^-\Sigma^-} = iA^6_{\Xi^-\Sigma^-}\,. \tag{24}
$$

## $\Xi \to \Xi$

$$
\begin{aligned}
A^3_{\Xi^0\Xi^0} = & -Z_\Xi \frac{a_D - a_F}{2} + \frac{4}{3}\Big[2(2t_3 - 2t_4 - t_7 + t_8)(M_K^2 - M_\pi^2) - 3(t_1 - t_2)(2M_K^2 + M_\pi^2)\Big] \\
& + \frac{I_M(M_\pi)}{(24F_0^2 m_0^2)}\Big[3(a_D - a_F)(4 + (D-F)^2)m_0^2 - (D-F)(-8\Delta a_D + 3(a_D - a_F)(D-F) + 8\Delta a_F)M_\pi^2\Big] \\
& + \frac{I_M(M_K)}{(36F_0^2 m_0^2)}\Big[3(-3a_F + 6a_F(D+F)^2 + a_D(3 + 2(D-3F)(D+F)))m_0^2 \\
& \qquad - 2(D\Delta a_D + 3\Delta a_D F + 3a_D(D-3F)(D+F) + 9a_F(D+F)^2 + 3D\Delta a_F - 3F\Delta a_F)M_K^2\Big] \\
& - \frac{I_M(M_\eta)}{(24F_0^2 m_0^2)}(a_D - a_F)(D+3F)^2(m_0^2 - M_\eta^2) \\
& - \frac{I_{MB}(M_\pi)}{(48F_0^2 m_0^2)}M_\pi^2(D-F)\Big[3(a_D - a_F)(D-F)(8m_0^2 - 5M_\pi^2) - 16(\Delta a_D - \Delta a_F)(4m_0^2 - M_\pi^2)\Big] \\
& - \frac{I_{MB}(M_K)}{(36F_0^2 m_0^2)}M_K^2\Big[3(D+F)(a_D(D-3F) + 3a_F(D+F))(8m_0^2 - 5M_K^2) \\
& \qquad + 2(3F(\Delta a_D - \Delta a_F) + D(\Delta a_D + 3\Delta a_F))(4m_0^2 - M_K^2)\Big] \\
& + \frac{I_{MB}(M_\eta)}{(48F_0^2 m_0^2)}M_\eta^2(a_D - a_F)(D+3F)^2(8m_0^2 - 5M_\eta^2) \\
& - \frac{I_{MBB}(0, M_\pi)}{(16F_0^2 m_0^2)}M_\pi^2(a_D - a_F)(D-F)^2(8m_0^4 - 12m_0^2 M_\pi^2 + 3M_\pi^4) \\
& - \frac{I_{MBB}(0, M_K)}{(12F_0^2 m_0^2)}M_K^2(D+F)(a_D(D-3F) + 3a_F(D+F))(8m_0^4 - 12m_0^2 M_K^2 + 3M_K^4) \\
& + \frac{I_{MBB}(0, M_\eta)}{(48F_0^2 m_0^2)}M_\eta^2(a_D - a_F)(D+3F)^2(8m_0^4 - 12m_0^2 M_\eta^2 + 3M_\eta^4) \\
& - \frac{1}{16\pi^2}\Big[(-54a_D D^2 + 54a_F D^2 + 72D\Delta a_D + 108a_D DF - 108a_F DF \\
& \qquad - 54a_D F^2 + 54a_F F^2 - 72F(\Delta a_D - \Delta a_F) - 72D\Delta a_F)\frac{M_\pi^4}{(432F_0^2 m_0^2)} \\
& \qquad + (27a_D D^2 - 27a_F D^2 - 12D\Delta a_D - 54a_D DF + 54a_F DF + 27a_D F^2 - 27a_F F^2 \\
& \qquad + 12F(\Delta a_D - \Delta a_F) + 12D\Delta a_F)\frac{M_\pi^6}{(432F_0^2 m_0^4)}\Big] \\
& - \frac{1}{16\pi^2}\Big[(-72a_D D^2 - 216a_F D^2 - 12D\Delta a_D + 144a_D DF - 432a_F DF \\
& \qquad + 216a_D F^2 - 216a_F F^2 - 36F(\Delta a_D - \Delta a_F) - 36D\Delta a_F)\frac{M_K^4}{(432F_0^2 m_0^2)} \\
& \qquad + (36a_D D^2 + 108a_F D^2 + 2D\Delta a_D - 72a_D DF + 216a_F DF \\
& \qquad - 108a_D F^2 + 108a_F F^2 + 6F(\Delta a_D - \Delta a_F) + 6D\Delta a_F)\frac{M_K^6}{(432F_0^2 m_0^4)}\Big] \\
& - \frac{1}{16\pi^2}\Big[(18a_D D^2 - 18a_F D^2 + 108a_D DF - 108a_F DF + 162a_D F^2 - 162a_F F^2)\frac{M_\eta^4}{(432F_0^2 m_0^2)} \\
& \qquad + (-9a_D D^2 + 9a_F D^2 - 54a_D DF + 54a_F DF - 81a_D F^2 + 81a_F F^2)\frac{M_\eta^6}{(432F_0^2 m_0^4)}\Big],
\end{aligned}
\tag{25}
$$

$$
\begin{aligned}
A^8_{\Xi^0\Xi^0} &= -Z_\Xi \frac{a_D + 3a_F}{2\sqrt{3}} - \frac{4}{3\sqrt{3}}\Big[2(10t_3 + 6t_4 + t_7 + 3t_8 + 6t_9)(M_K^2 - M_\pi^2) + 3(t_1 + 3t_2)(2M_K^2 + M_\pi^2)\Big] \\
&+ \frac{I_M(M_\pi)}{(8F_0^2 m_0^2)}\sqrt{3}(a_D + 3a_F)(D - F)^2(-m_0^2 + M_\pi^2) \\
&+ \frac{I_M(M_K)}{(12\sqrt{3}F_0^2 m_0^2)}\Big[(27a_F + a_D(9 + 8D(D + 3F)))m_0^2 - 2(5D\Delta a_D + 3\Delta a_D F + 4a_D D(D + 3F) + 3D\Delta a_F + 9F\Delta a_F)M_K^2\Big] \\
&- \frac{I_M(M_\eta)}{(24\sqrt{3}F_0^2 m_0^2)}(a_D + 3a_F)(D + 3F)^2(m_0^2 - M_\eta^2) \\
&+ \frac{I_{MB}(M_\pi)}{(16F_0^2 m_0^2)}\sqrt{3}M_\pi^2(a_D + 3a_F)(D - F)^2(8m_0^2 - 5M_\pi^2) \\
&+ \frac{I_{MB}(M_K)}{(6\sqrt{3}F_0^2 m_0^2)}M_K^2\Big[(5D\Delta a_D + 3\Delta a_D F + 3D\Delta a_F + 9F\Delta a_F)(-4m_0^2 + M_K^2) + 2a_D D(D + 3F)(-8m_0^2 + 5M_K^2)\Big] \\
&+ \frac{I_{MB}(M_\eta)}{(48\sqrt{3}F_0^2 m_0^2)}M_\eta^2(a_D + 3a_F)(D + 3F)^2(8m_0^2 - 5M_\eta^2) \\
&+ \frac{I_{MBB}(0, M_\pi)}{(16F_0^2 m_0^2)}\sqrt{3}M_\pi^2(a_D + 3a_F)(D - F)^2(8m_0^4 - 12m_0^2 M_\pi^2 + 3M_\pi^4) \\
&- \frac{I_{MBB}(0, M_K)}{(3\sqrt{3}F_0^2 m_0^2)}M_K^2 a_D D(D + 3F)(8m_0^4 - 12m_0^2 M_K^2 + 3M_K^4) \\
&+ \frac{I_{MBB}(0, M_\eta)}{(48\sqrt{3}F_0^2 m_0^2)}M_\eta^2(a_D + 3a_F)(D + 3F)^2(8m_0^4 - 12m_0^2 M_\eta^2 + 3M_\eta^4) \\
&- \frac{1}{16\pi^2}\left[\frac{\sqrt{3}(a_D + 3a_F)(D - F)^2 M_\pi^4}{(8F_0^2 m_0^2)} - \frac{\sqrt{3}(a_D + 3a_F)(D - F)^2 M_\pi^6}{(16F_0^2 m_0^4)}\right] \\
&- \frac{1}{16\pi^2}\Big[(-96a_D D(D + 3F) - 12(5D\Delta a_D + 3\Delta a_D F + 3D\Delta a_F + 9F\Delta a_F))\frac{M_K^4}{(144\sqrt{3}F_0^2 m_0^2)} \\
&\qquad + (48a_D D(D + 3F) + 2(5D\Delta a_D + 3\Delta a_D F + 3D\Delta a_F + 9F\Delta a_F))\frac{M_K^6}{(144\sqrt{3}F_0^2 m_0^4)}\Big] \\
&- \frac{1}{16\pi^2}\left[\frac{(a_D + 3a_F)(D + 3F)^2 M_\eta^4}{(24\sqrt{3}F_0^2 m_0^2)} - \frac{(a_D + 3a_F)(D + 3F)^2 M_\eta^6}{(48\sqrt{3}F_0^2 m_0^4)}\right].
\end{aligned}
\tag{26}
$$

$$
A^3_{\Xi^-\Xi^-} = A^1_{\Xi^-\Xi^0} = -A^3_{\Xi^0\Xi^0}\,, \quad A^2_{\Xi^-\Xi^0} = iA^1_{\Xi^-\Xi^0}\,, \qquad A^8_{\Xi^-\Xi^-} = A^8_{\Xi^0\Xi^0}\,. \tag{27}
$$

## Singlet results in the nucleon sector

$$
\begin{aligned}
A^s_{pp}(0) = {} & Z_N\frac{a_s}{2} + \frac{M_\pi^2\left(18a_s(D+F)^2+512\pi^2F_0^2(3t_{11}-2t_{12}+6t_{13})\right)}{384\pi^2F_0^2} \\
& + \frac{3a_s(D+F)^2M_\pi^2\left(3m_0^4-6m_0^2M_\pi^2+2M_\pi^4\right)\mathrm{Log}\left[\frac{M_\pi}{m_0}\right]}{64\pi^2F_0^2m_0^4} \\
& - \frac{3a_s(D+F)^2M_\pi^3\left(5m_0^4-5m_0^2M_\pi^2+M_\pi^4\right)\mathrm{ArcCos}\left[-\frac{M_\pi}{2m_0}\right]}{32\pi^2F_0^2m_0^5\sqrt{4-\frac{M_\pi^2}{m_0^2}}} \\
& - \frac{3a_s\left(D+F\right)^2M_\pi^6}{128\pi^2F_0^2m_0^4} \\
& + \frac{M_K^2\left(4a_s(5D^2-6DF+9F^2)+1024\pi^2F_0^2(3t_{11}+t_{12}-3t_{13})\right)}{384\pi^2F_0^2} \\
& + \frac{a_s\left(5D^2-6DF+9F^2\right)M_K^2\left(3m_0^4-6m_0^2M_K^2+2M_K^4\right)\mathrm{Log}\left[\frac{M_K}{m_0}\right]}{96\pi^2F_0^2m_0^4} \\
& - \frac{a_s\left(5D^2-6DF+9F^2\right)M_K^3\left(5m_0^4-5m_0^2M_K^2+M_K^4\right)\mathrm{ArcCos}\left[-\frac{M_K}{2m_0}\right]}{48\pi^2F_0^2m_0^5\sqrt{4-\frac{M_K^2}{m_0^2}}} \\
& - \frac{a_s\left(5D^2-6DF+9F^2\right)M_K^6}{192\pi^2F_0^2m_0^4} \\
& + \frac{a_s\left(D-3F\right)^2M_\eta^2}{192\pi^2F_0^2} + \frac{a_s(D-3F)^2M_\eta^2\left(3m_0^4-6m_0^2M_\eta^2+2M_\eta^4\right)\mathrm{Log}\left[\frac{M_\eta}{m_0}\right]}{192\pi^2F_0^2m_0^4} \\
& - \frac{a_s(D-3F)^2M_\eta^3\left(5m_0^4-5m_0^2M_\eta^2+M_\eta^4\right)\mathrm{ArcCos}\left[-\frac{M_\eta}{2m_0}\right]}{96\pi^2F_0^2m_0^5\sqrt{4-\frac{M_\eta^2}{m_0^2}}} - \frac{a_s\left(D-3F\right)^2M_\eta^6}{384\pi^2F_0^2m_0^4}\,.
\end{aligned}
\tag{28}
$$

Again, using isospin symmetry one finds $A^s_{nn} = A^s_{pp}$ .

## 3 Loop functions

In the last section, we have used the following abbreviations for the loop functions:

$$I_M(M) = \frac{M^2}{8\pi^2} \ln\alpha\,, \tag{29}$$

where $\alpha = M/m_0$ . Note that we use $\mu = m_0$ for the renormalization scale everywhere, following the original proposal of Infrared Regularization by Becher and Leutwyler. Furthermore,

$$I_{MB}(M) = \frac{1}{16\pi^2}((2\ln\alpha - 1)\frac{\alpha^2}{2} + \alpha\sqrt{4-\alpha^2}\arccos(-\frac{\alpha}{2}))\,. \tag{30}$$

Moreover, the renormalized three-point function in Infrared Regularization, taken at $\Delta^2 = 0$, is given by

$$I_{MBB}(0,M) = -\frac{1}{32\pi^2 m_0^2}\left(2\ln\alpha + 1 - \frac{2\alpha}{\sqrt{4-\alpha^2}}\arccos(-\frac{\alpha}{2})\right)\,. \tag{31}$$

The baryon wave function renormalization factors are, at the one-loop level:

$$\begin{aligned}
Z_N = {} & 1 - M_\pi^2\frac{3(D+F)^2}{(32\pi^2F_0^2)} - M_K^2\frac{5D^2-6DF+9F^2}{(48\pi^2F_0^2)} - M_\eta^2\frac{(D-3F)^2}{(96\pi^2F_0^2)} \\
& - \frac{3(D+F)^2M_\pi^3(-3m_0^2+M_\pi^2)}{(16\pi^2F_0^2m_0^3\sqrt{4-\frac{M_\pi^2}{m_0^2}})}\arccos\left(-\frac{M_\pi}{2m_0}\right) \\
& - \frac{(5D^2-6DF+9F^2)M_K^3(-3m_0^2+M_K^2)}{(24\pi^2F_0^2m_0^3\sqrt{4-\frac{M_K^2}{m_0^2}})}\arccos\left(-\frac{M_K}{2m_0}\right) \\
& - \frac{(D-3F)^2M_\eta^3(-3m_0^2+M_\eta^2)}{(48\pi^2F_0^2m_0^3\sqrt{4-\frac{M_\eta^2}{m_0^2}})}\arccos\left(-\frac{M_\eta}{2m_0}\right) \\
& + \frac{3(D+F)^2M_\pi^2(-3m_0^2+2M_\pi^2)}{(32\pi^2F_0^2m_0^2)}\log\left(\frac{M_\pi}{m_0}\right) \\
& + \frac{(5D^2-6DF+9F^2)M_K^2(-3m_0^2+2M_K^2)}{(48\pi^2F_0^2m_0^2)}\log\left(\frac{M_K}{m_0}\right) \\
& + \frac{(D-3F)^2M_\eta^2(-3m_0^2+2M_\eta^2)}{(96\pi^2F_0^2m_0^2)}\log\left(\frac{M_\eta}{m_0}\right)\,,
\end{aligned} \tag{32}$$

$$
\begin{aligned}
Z_\Lambda = {} & 1 - M_\pi^2 \frac{D^2}{(8\pi^2 F_0^2)} - M_K^2 \frac{D^2 + 9F^2}{(24\pi^2 F_0^2)} - M_\eta^2 \frac{D^2}{(24\pi^2 F_0^2)} \\
& + \frac{D^2(3m_0^2 M_\pi^3 - M_\pi^5)}{(4\pi^2 F_0^2 m_0^3 \sqrt{4 - \frac{M_\pi^2}{m_0^2}})} \arccos\left(-\frac{M_\pi}{2m_0}\right) \\
& - \frac{(D^2 + 9F^2) M_K^3 (-3m_0^2 + M_K^2)}{(12\pi^2 F_0^2 m_0^3 \sqrt{4 - \frac{M_K^2}{m_0^2}})} \arccos\left(-\frac{M_K}{2m_0}\right) \\
& + \frac{D^2(3m_0^2 M_\eta^3 - M_\eta^5)}{(12\pi^2 F_0^2 m_0^3 \sqrt{4 - \frac{M_\eta^2}{m_0^2}})} \arccos\left(-\frac{M_\eta}{2m_0}\right) \\
& + \frac{D^2(-3m_0^2 M_\pi^2 + 2M_\pi^4)}{(8\pi^2 F_0^2 m_0^2)} \log\left(\frac{M_\pi}{m_0}\right) \\
& + \frac{(D^2 + 9F^2) M_K^2 (-3m_0^2 + 2M_K^2)}{(24\pi^2 F_0^2 m_0^2)} \log\left(\frac{M_K}{m_0}\right) \\
& + \frac{D^2(-3m_0^2 M_\eta^2 + 2M_\eta^4)}{(24\pi^2 F_0^2 m_0^2)} \log\left(\frac{M_\eta}{m_0}\right) \,,
\end{aligned}
\tag{33}
$$

$$
\begin{aligned}
Z_\Sigma = {} & 1 - M_\pi^2 \frac{D^2 + 6F^2}{(24\pi^2 F_0^2)} - M_K^2 \frac{D^2 + F^2}{(8\pi^2 F_0^2)} - M_\eta^2 \frac{D^2}{(24\pi^2 F_0^2)} \\
& - \frac{(D^2 + 6F^2) M_\pi^3 (-3m_0^2 + M_\pi^2)}{(12\pi^2 F_0^2 m_0^3 \sqrt{4 - \frac{M_\pi^2}{m_0^2}})} \arccos\left(-\frac{M_\pi}{2m_0}\right) \\
& - \frac{(D^2 + F^2) M_K^3 (-3m_0^2 + M_K^2)}{(4\pi^2 F_0^2 m_0^3 \sqrt{4 - \frac{M_K^2}{m_0^2}})} \arccos\left(-\frac{M_K}{2m_0}\right) \\
& + \frac{D^2(3m_0^2 M_\eta^3 - M_\eta^5)}{(12\pi^2 F_0^2 m_0^3 \sqrt{4 - \frac{M_\eta^2}{m_0^2}})} \arccos\left(-\frac{M_\eta}{2m_0}\right) \\
& + \frac{(D^2 + 6F^2) M_\pi^2 (-3m_0^2 + 2M_\pi^2)}{(24\pi^2 F_0^2 m_0^2)} \log\left(\frac{M_\pi}{m_0}\right) \\
& + \frac{(D^2 + F^2) M_K^2 (-3m_0^2 + 2M_K^2)}{(8\pi^2 F_0^2 m_0^2)} \log\left(\frac{M_K}{m_0}\right) \\
& + \frac{D^2(-3m_0^2 M_\eta^2 + 2M_\eta^4)}{(24\pi^2 F_0^2 m_0^2)} \log\left(\frac{M_\eta}{m_0}\right) \,,
\end{aligned}
\tag{34}
$$

$$
\begin{aligned}
Z_{\Xi} = {} & 1 - M_\pi^2 \frac{3(D-F)^2}{(32\pi^2 F_0^2)} - M_K^2 \frac{5D^2+6DF+9F^2}{(48\pi^2 F_0^2)} - M_\eta^2 \frac{(D+3F)^2}{(96\pi^2 F_0^2)} \\
& - \frac{3(D-F)^2 M_\pi^3 (-3m_0^2 + M_\pi^2)}{(16\pi^2 F_0^2 m_0^3 \sqrt{4 - \frac{M_\pi^2}{m_0^2}})} \arccos\left(-\frac{M_\pi}{2m_0}\right) \\
& - \frac{(5D^2+6DF+9F^2) M_K^3 (-3m_0^2 + M_K^2)}{(24\pi^2 F_0^2 m_0^3 \sqrt{4 - \frac{M_K^2}{m_0^2}})} \arccos\left(-\frac{M_K}{2m_0}\right) \\
& - \frac{(D+3F)^2 M_\eta^3 (-3m_0^2 + M_\eta^2)}{(48\pi^2 F_0^2 m_0^3 \sqrt{4 - \frac{M_\eta^2}{m_0^2}})} \arccos\left(-\frac{M_\eta}{2m_0}\right) \\
& + \frac{3(D-F)^2 M_\pi^2 (-3m_0^2 + 2M_\pi^2)}{(32\pi^2 F_0^2 m_0^2)} \log\left(\frac{M_\pi}{m_0}\right) \\
& + \frac{(5D^2+6DF+9F^2) M_K^2 (-3m_0^2 + 2M_K^2)}{(48\pi^2 F_0^2 m_0^2)} \log\left(\frac{M_K}{m_0}\right) \\
& + \frac{(D+3F)^2 M_\eta^2 (-3m_0^2 + 2M_\eta^2)}{(96\pi^2 F_0^2 m_0^2)} \log\left(\frac{M_\eta}{m_0}\right) .
\end{aligned}
\tag{35}
$$
